# Supplementary material for: Multi-Draft Speculative Sampling: Canonical Decomposition and Theoretical Limits
Source: arXiv:2410.18234 source file (2025-05-08)
Supplement: Supplementary file 1 [file truncVoc.tex]

Recall that $\Omega =\{1,\ldots, n\}$ denotes the full vocabulary and $\Omega_0\subseteq \Omega$ is a high probability set of tokens selected so that $q(\Omega_0) = 1-q_\eps$ and $p(\Omega_0) =1-p_\eps$.  Recall that  $\tilde{p}(\cdot)$ and $\tilde{q}(\cdot)$ denote the distributions over $\Omega_0$ obtained by truncating $p(\cdot)$ and $q(\cdot)$ to $\Omega_0$  and re-normalizing them. 

Given the set of input tokens $\cS =\{X_1,\ldots, X_K\}$ we select a subset $\tilde{\cS} \subseteq \cS$ by discarding any tokens in $\cS$ that do not belong to $\Omega$. Let $\{\tilde{X}_1, \ldots, \tilde{X}_{K'}\}$ denote the tokens in $\tilde{S}$, which are effectively sampled from the distribution $\tilde{p}(\cdot)$ i.e., $\Pr(\tilde{X}_i = x)= \tilde{p}(x)$ if $x \in \Omega_0$.

We then perform importance weighted sampling over the input tokens $\tilde{\cS}$ to generate output token $Y \sim p_I(\cdot)$. We then perform speculative sampling using target distribution $q(\cdot)$ and output the resulting token $Z \sim q(\cdot)$.

Let $\tilde{P}_{\Omega_0}(\mrm{acc})$ be the acceptance probability of the proposed truncated alphabet scheme and 
$\tilde{P}^\star(\mrm{acc})$ be the optimal acceptance probability without truncation of the alphabet. 

Without loss of generality assume $\Omega_0 = \{1,2,\ldots, \delta\}$ and $\Omega = \{1,2,\ldots, n\}$. Also assume $p(\Omega_0) = 1-p_\eps$ and $q(\Omega_0)=1-q_\eps$. Let $\cS = \{X_1, X_2\}$ denote the input tokens and $\tilde{\cS}$ denote the  tokens that are in $\Omega_0$.

We consider the following:
\begin{align}
 &\tilde{P}_{\Omega_0}(\mrm{acc}~|~\tilde{\cS}= \cS) = \sum_{i\in \Omega_0} \min (q_i, \tilde{p}_I(i))
\end{align}
where 
\begin{align}
    \tilde{p}_I(i) = \tilde{p}_i^2 + \sum_{j=1, j\neq i}^{\del} 2 \tilde{p}_i \tilde{p}_j \tilde{w}_{i,j} 
    \label{eq:p-align0}
\end{align}
where $\tilde{w}_{m,n}$ are the associated variables as discussed in our formulation.  

When truncation is not used, let $w_{i,j}$ be the associated variables for $i,j\in \Omega$ and $i\neq j$ such that
\begin{align}
    p_I(i) = p_i^2 + \sum_{j=1, j\neq i}^{n} 2p_i p_j w_{i,j} 
\end{align}
achieves the optimal acceptance probability: 
\begin{align}
    P^\star(\mrm{acc}) = \sum_{i=1}^n \min(p_I(i), q_i) \le \sum_{i=1}^\delta \min(p_I(i),q_i) + q_\epsilon 
\end{align}

In the optimization program~\eqref{eq:p-align0}, we consider a potentially sub-optimal choice:: $\tilde{w}_{i,j}=w_{i,j}$ for $i<j$. Also note that due to truncation, $\tilde{p}_i = p_i/p(\Omega_0) \ge p_i$ for each $i=1,2,\ldots, \delta$. Thus it follows that
\begin{align}
    \tilde{p}_I(i) \ge p_I(i), \quad \forall i\in \Omega_0
    \label{eq:p-align}
\end{align}
It thus follows that:
\begin{align}
  &P^\star(\mrm{acc}) \le  \sum_{i=1}^\delta \min(\tilde{p}_I(i),q_i) + q_\epsilon  \\
  &\le \tilde{P}^\star(\mrm{acc}|\tilde{\cS}= \cS) + q_\epsilon
\end{align}
and:\begin{align}
& \tilde{P}^\star(\mrm{acc}) \ge     \Pr(\tilde{\cS}= \cS) \cdot\tilde{P}^\star(\mrm{acc}|\tilde{\cS}= \cS) \\
&\prod_{i=1}^2 P(X_i \in \cS) \Pr(\tilde{\cS}= \cS) \cdot\tilde{P}^\star(\mrm{acc}|\tilde{\cS}= \cS) \\
&=(1-p_\eps)^2\left(P^\star(\mrm{acc})-q_\epsilon\right)\\
&\ge (1-2p_\eps)\left(P^\star(\mrm{acc}) - q_\eps) \right)
\end{align}
